# Supplementary material for: Supervised domain adaptation for building extraction from off-nadir aerial images
Source: arXiv:2311.03867 source file (2024-08-07)
Supplement: Supplementary file 1 [file SupplementaryMaterial.pdf]

# Supplementary Material

Bipul Neupane<sup>a,b,\*</sup>, Jagannath Aryal<sup>a,b</sup>, Abbas Rajabifard<sup>b</sup>

<sup>a</sup>Earth Observation and AI Research Group, Faculty of Engineering and IT, The University of Melbourne, Parkville, Melbourne, 3010, VIC, Australia

<sup>b</sup>Department of Infrastructure Engineering, Faculty of Engineering and IT, The University of Melbourne, Parkville, Melbourne, 3010, VIC, Australia

## Abstract

This document is provided as a supplementary material for the paper titled “Supervised domain adaptation for building extraction from off-nadir aerial images”. The document provides the detailed explanation of how the experiments with knowledge distillation (KD) and deep mutual learning (DML) are set up. Furthermore, it also provides a grid search of the “temperature” hyperparameter that controls the “softness” of the Teacher’s prediction during the distillation of Student.

## 1. Setup for Knowledge Distillation

KD, as introduced by (Hinton et al., 2015), is a technique for compressing knowledge from a large, complex model into a smaller, deployable model while minimising the loss in performance. In the context of cross-modal distillation, where a Teacher network is trained on noisy samples and a Student network on clean ones (Xu et al., 2022), we employ a similar approach of KD in our work. The Teacher is trained on the noise-unaccounted T dataset. It yields subpar building segmentation results in the presence of noisy label types but excels in the case of noise-lacking building types due to its exposure to a vast dataset. The loss of the Teacher can be formulated with the loss function such as Dice loss (Sudre et al., 2017). In the paper, we use the loss function identified from the hyperparameter search.

An illustrative example of KD with a Teacher and a Student of EDN configurations is depicted in Figure 1. The Student is trained using a cleaner, smaller dataset S, aiming to replicate the Teacher’s performance. The training involves a distillation loss, which is a combination of a traditional loss (like cross-entropy against the true labels) and the KD loss that aligns the Student’s predictions with the Teacher’s soft targets. This collaborative process empowers the Student to overcome the challenges posed by noisy labels while also acquiring the ability to accurately extract buildings without mislabeling the classes found in the Teacher.

The total loss function for the Student can be expressed as

$$L_{total} = \alpha L_{search} + (1 - \alpha) L_{distil} \quad (1)$$

$$L_{search} = L_{seg} \text{ (from hyperparameter search)} \quad (2)$$

where  $L_{search}$  is the loss function determined from the hyperparameter search, focusing on the segmentation loss  $L_{seg}$  such

as *Dice Loss* between GT and the Student’s predictions. The  $\alpha$  hyperparameter balances the focus between segmentation accuracy ( $L_{search}$ ) and fidelity to the Teacher’s multi-scale feature maps, which is distillation loss, formulated to reduce differences in multi-scale feature maps through:

$$L_{distil} = L_{MSE} \left( \sigma \left( p_j^t / \tau \right), \sigma \left( p_j^s / \tau \right) \right) \quad (3)$$

where  $L_{MSE}$  denotes the Mean Square Error Loss,  $p_j^t$  and  $p_j^s$  represent the Teacher’s and Student’s predictions for the  $j^{th}$  pixel,  $\sigma$  denotes the sigmoid activation function, and temperature ( $\tau$ ) is the hyperparameter controlling the softness of the distributions. The  $\tau$  parameter is identified in this study from a grid search in 3.  $L_{MSE}$  is defined as the average squared difference between the GT and prediction for each pixel:

$$L_{MSE} = \frac{1}{N} \sum_{i=1}^N (y_j - p_j)^2 \quad (4)$$

where  $y_j$  and  $p_j$  respectively denote the GT and prediction for  $j^{th}$  pixel,  $\frac{1}{N}$  is the normalisation factor used to compute the average squared difference.

This loss function framework above ensures that the Student not only learns to accurately segment the images, similar to the Teacher but also aligns its internal feature representations with those of the Teacher. The integration of  $L_{distil}$  specifically targets the preservation of spatial hierarchies and textures learned by the Teacher, crucial for tasks like building segmentation amidst noisy data. By optimising the composite total loss, the Student model inherits the Teacher’s robustness and high performance, achieving effective model compression without significant loss in accuracy, even when trained on a limited set of clean-labeled samples. This methodology underscores the adaptability of KD techniques in addressing the challenges of noisy labels and the need for model efficiency in deployment scenarios.

To formulate the network configurations of the Teacher, this paper investigates the EDNs with the best trade-off between size and evaluation scores. Then various Student networks with

\*Corresponding author

Email addresses: bneupane@student.unimelb.edu.au (Bipul Neupane), jagannath.aryal@unimelb.edu.au (Jagannath Aryal), abbas.r@unimelb.edu.au (Abbas Rajabifard)

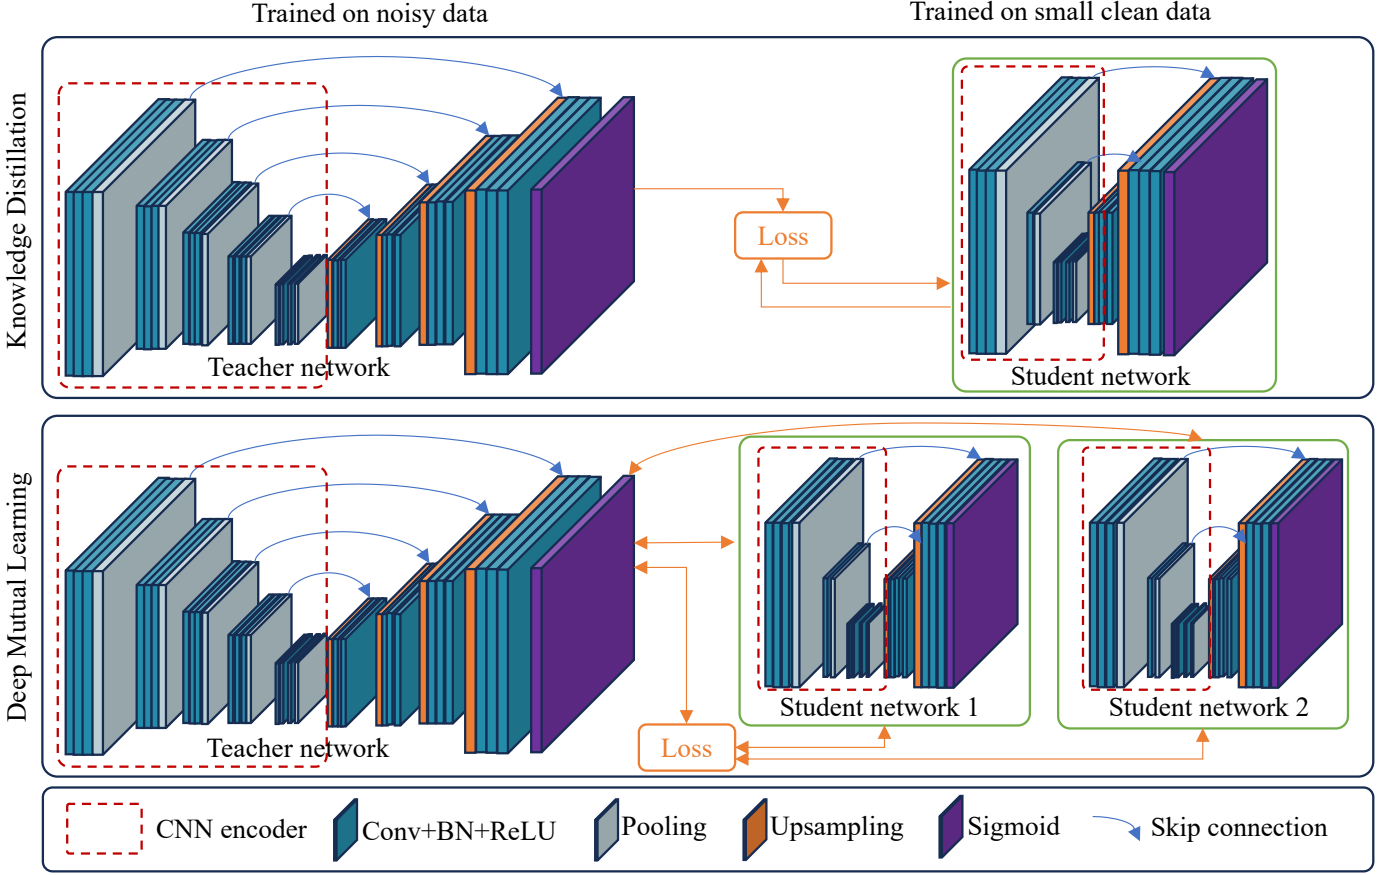

Figure 1: Illustrative example of KD and DML. (a) KD of a Teacher network trained on noisy data to Student network distilled on a small clean data. (b) DML between one Teacher network trained on noisy data and two Student networks that are collaboratively distilled on the small clean data.

lower network parameters (size) are explored to achieve model compression.

## 2. Setup for Deep Mutual Learning

DML (Zhang et al., 2018) is a strategy where learning is not a one-way transfer from a Teacher to a Student model, but rather a collaborative process where multiple Students learn together by teaching each other throughout the training process. For the simplicity of the investigation, we involve one Teacher and two Students, where the DML framework facilitates a dynamic learning environment where all models benefit and improve by learning from each other's predictions in addition to learning from the GT.

An illustrative example of DML with a Teacher and two Students of EDN configurations is depicted in Figure 1. In our setup of DML, each model (the Teacher and both Students) is trained not only to perform well on the task at hand (segmentation) but also to mimic the predictions of the other models. This is achieved through a combination of task-specific loss (such as dice loss for segmentation accuracy) and distillation loss, which in this context is extended to mutual distillation loss among the Student networks.

To describe the model training in DML, each model  $M_k$  (where  $k$  can denote the Teacher or any Student) is trained using a loss function that comprises two components: the task-specific loss from the hyperparameter search (e.g., dice loss) for direct learning from the GT labels, and a mutual distillation loss that encourages each model to learn from the predictions of the other models. The total loss for model  $M_k$  is given by:

$$L_{total}^{(k)} = \alpha L_{search}^{(k)} + \frac{1 - \alpha}{K} \sum_{i=1, i \neq k}^K L_{distil}^{(k,i)} \quad (5)$$

where  $L_{search}^{(k)}$  is the loss from the hyperparameter search for model  $M_k$ ,  $L_{distil}^{(k,i)}$  is the mutual distillation loss between model  $M_k$  and another model  $M_i$ , computed for all  $K$  models in the training setup except for  $k$ . The  $\alpha$  is a hyperparameter balancing the importance of the segmentation loss against the mutual distillation loss.

The mutual distillation loss between models  $M_k$  and  $M_i$  is designed to minimise the discrepancy in their predictions, encouraging each model to learn from the others. It can be formulated as an MSE loss over their predictions, adjusted by a temperature  $\tau$  for softening:

$$L_{distil}^{(k,i)} = L_{MSE}(\sigma(p_j^k/\tau), \sigma(p_j^i/\tau)) \quad (6)$$

where  $p_j^k$  and  $p_j^i$  are the predictions for the  $j^{th}$  pixel from models  $M_k$  and  $M_i$ , respectively, and  $\sigma$  denotes the sigmoid activation function. The  $\tau$  is used as identified from the investigation in 3.

Students achieve a consensus on correct predictions among each other with the loss setup above, which enhances their generalising ability and robustness. DML is valuable when dealing with limited labelled data such as our dataset S.

### 3. Identifying best temperature for knowledge distillation

Temperature ( $\tau$ ) is a hyperparameter used to soften the outputs (predictions) of the Teacher, which are then used to distil the Student network. A grid search is performed with several  $\tau$  values ranging from 1 to 9 during the KD of U-VGG19, U-EfficientNetv2B3, and U-TinyNet-e. We report only the odd values of  $\tau$  to keep the experiments short. The results are shown in Figure 2. The  $\tau$  of 7, 3, and 5 serves best for U-VGG19, U-EfficientNetv2B3, and U-TinyNet-e respectively, yielding the least loss.  $\tau$  values that yield the least loss are used in the experiments of KD and DML.

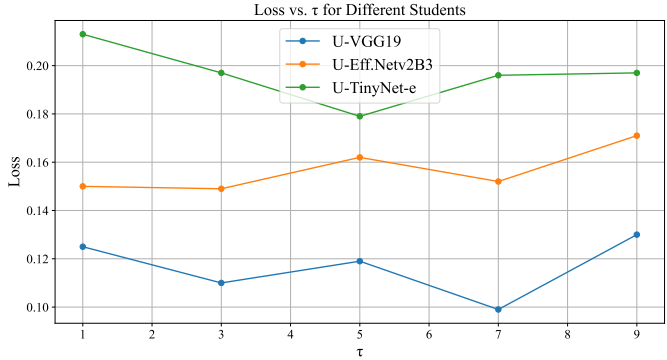

Figure 2: Grid search to identify the best temperature ( $\tau$ ) for KD and DML. Three Students are distilled in the S-S setting for the  $\tau$  of every other value from 1 to 9.

### References

- Hinton, G., Vinyals, O., Dean, J., et al. (2015). Distilling the knowledge in a neural network. *arXiv preprint arXiv:1503.02531*, 2(7).
- Sudre, C. H., Li, W., Vercauteren, T., Ourselin, S., and Jorge Cardoso, M. (2017). Generalised dice overlap as a deep learning loss function for highly unbalanced segmentations. In *Deep learning in medical image analysis and multimodal learning for clinical decision support*, pages 240–248. Springer.
- Xu, G., Deng, M., Sun, G., Guo, Y., and Chen, J. (2022). Improving building extraction by using knowledge distillation to reduce the impact of label noise. *Remote Sensing*, 14(22):5645.
- Zhang, Y., Xiang, T., Hospedales, T. M., and Lu, H. (2018). Deep mutual learning. In *Proceedings of the IEEE conference on computer vision and pattern recognition*, pages 4320–4328.
